# Supplementary material for: Time-Reversal Symmetry in RDMFT and pCCD with Complex-Valued Orbitals
Source: arXiv:2410.03620 source file (2024-12-09)
Supplement: Supplementary file 1 [file si_name.pdf]

# Supporting Information for: Time-Reversal Symmetry in RDMFT and pCCD with Complex-Valued Orbitals

Mauricio Rodríguez-Mayorga,*,† Pierre-François Loos,¶ Fabien Bruneval,§ and Lucas Visscher‡

†*Grenoble Alpes University, CNRS, Grenoble INP, Institut Néel, 25 rue des Martyrs, 38042 Grenoble, France*

‡*Theoretical Chemistry, Vrije Universiteit, De Boelelaan 1108, 1081 HZ Amsterdam, The Netherlands*

¶*Laboratoire de Chimie et Physique Quantiques (UMR 5626), Université de Toulouse, CNRS, UPS, France*

§*Université Paris-Saclay, CEA, Service de recherche en Corrosion et Comportement des Matériaux, SRMP, 91191 Gif-sur-Yvette, France*

E-mail: marm3.14@gmail.com

## 1 When the complex (with time-reversal symmetry) and the real solutions coincide. The $H_2$ example.

For two-electron systems, the PNOF$i$ ($i = 5, 6,$ and 7), as well as the pCCD approximation, coincide with the so-called fixed-phase RDMFT functional[1] of Shull and Löwdin that is known to reproduce the exact full CI (FCI) energy for two-electron systems.[2] In Fig. 1,

we have plotted the potential energy curves (PECs) for the $H_2$ system. Our results indicate that the RPNOF5 and the TPNOF5 coincide for all correlation regimes. This is because the PNOF5 functional reproduces the FCI results and the use of complex coefficients in constructing the spin-down orbitals does not introduce any extra degrees of freedom/flexibility making both solutions coincide. The eigenvalues of the complex Hessian matrix [see Eq. (**??**)] constructed using the real optimized orbitals (multiplied by random phases) and fixed occupations numbers along the PEC shows that all the eigenvalues are positive, which proves that the real solutions are also a minimum for the complex orbital optimization problem.

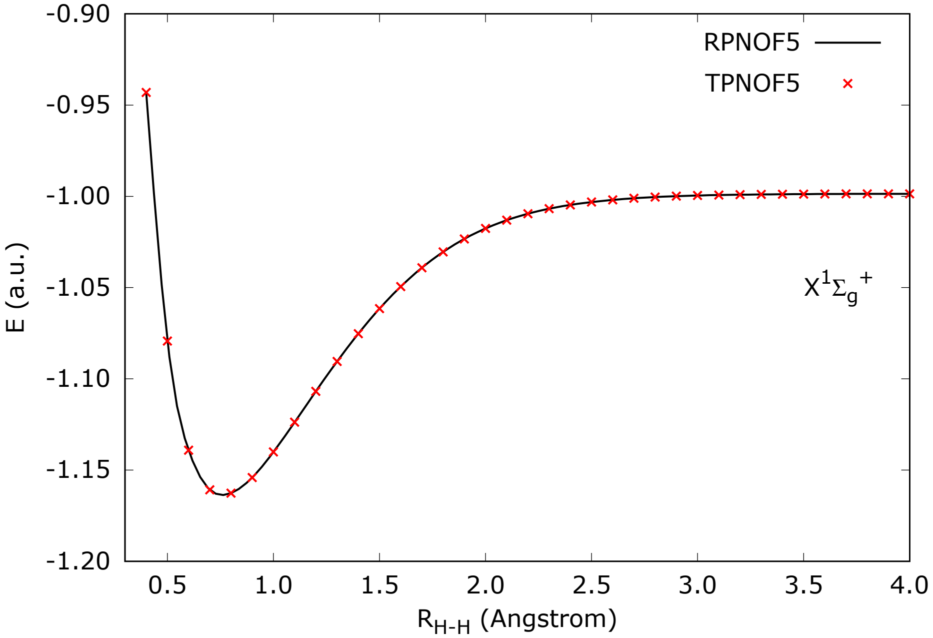


Figure 1: Potential energy curves obtained with the real (black solid) and complex (red crosses) versions of the PNOF5 functional for the dissociation of the $H_2$ molecule.

## 2 The $BeH_2$ pCCD and PNOF5 results.

In general, the PNOF5 and the pCCD are very similar. Let us recall that PNOF5 corresponds to an anti-symmetrized product of strongly orthogonal geminal (APSG) wavefunction.[3] And, the APSG is closely related to the pCCD wavefunction produced by the exponential ansatz.

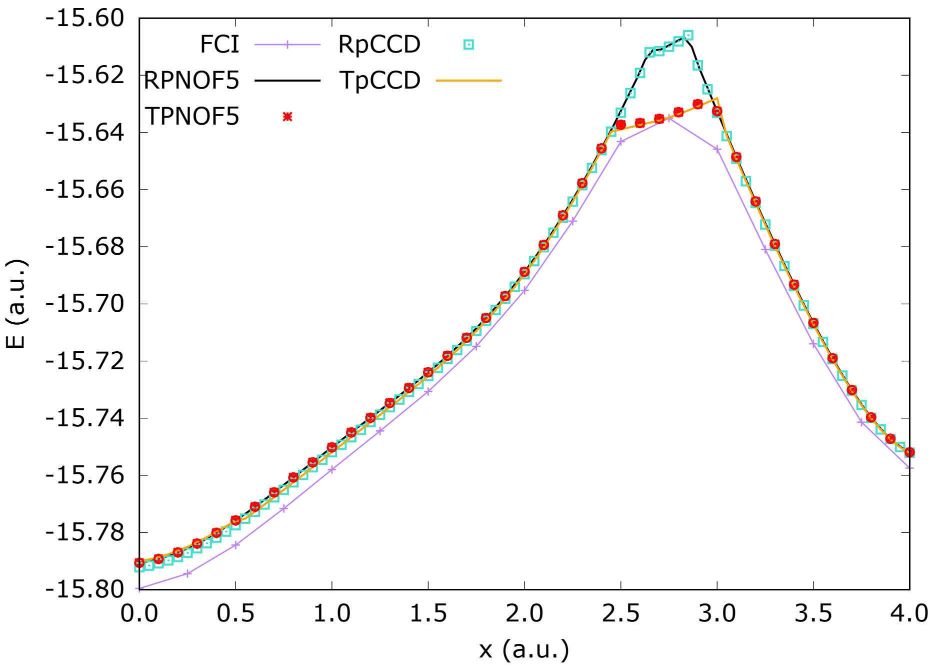


Figure 2: For the $BeH_2$ system, we present the FCI, PNOF5, and pCCD potential energy curves

To facilitate the convergence to the lowest energy state using the pCCD method, the PNOF5 and the GNOF orbitals were used as a starting point for these calculations. Moreover, in the interval $x \in [2.5; 3.5]$, the $x = 2.75$ geometry was computed first and then we scanned backward and forward the rest of the geometries. Finally, let us remark that pCCD also produces energies above the FCI results, which indicates that this method does not introduce $N$-representability violations.

# References


(1) Shull, H.; Löwdin, P.-O. Superposition of configurations and natural spin orbitals. Applications to the He problem. *J. Chem. Phys.* **1959**, *30*, 617.

(2) Rodríguez-Mayorga, M.; Ramos-Cordoba, E.; Via-Nadal, M.; Piris, M.; Matito, E. Comprehensive benchmarking of density matrix functional approximations. *Phys. Chem. Chem. Phys.* **2017**, *19*, 24029.

(3) Pernal, K. The equivalence of the Piris Natural Orbital Functional 5 (PNOF5) and the antisymmetrized product of strongly orthogonal geminal theory. *Comput. Theor. Chem.* **2013**, *1003*, 127–129.
